# Supplementary material for: Improving Web Content Blocking With Event-Loop-Turn Granularity JavaScript Signatures
Source: arXiv:2005.11910 source file (2020-05-25)
Supplement: Supplementary file 1 [file X_appendix.tex]

\appendix
\section{Complete Browser Instrumentation Points}
\label{sec:appendix}

\begin{table}
  \begin{tabular}{l}
    \toprule
      DOM Events \\
    \midrule
      \ctab{} node creation \\
      \ctab{} node insertion \\
      \ctab{} node deletion \\
      \ctab{} node modification \\
      \ctab{} script executions \\
      \ctab{} frame creations \\
      \ctab{} operations in local (i.e. same domain) frames \\
    \midrule
      Network requests \\
    \midrule
      \ctab{} AJAX API \\
      \ctab{} Fetch API \\
      \ctab{} DOM-related (e.g. \texttt{<img scr=X>}) \\
    \midrule
      \JS{} Builtin APIs \\
    \midrule
      \ctab{} date APIs \\
      \ctab{} timer APIs \\
      \ctab{} event registrations \\
    \midrule
      Web APIs \\
    \midrule
      \ctab{} storage APIs (\\
      \ctab{} \ctab{} \texttt{document.cookie}, \texttt{localStorage}, \texttt{sessionStorage}) \\
      \ctab{} APIs used by browser fingerprinting scripts (e.g. \\
      \ctab{} \ctab{} \texttt{navigator.\{platform, userAgent, language\}, etc}, \\
      \ctab{} \ctab{} \texttt{screen.\{height, width, colorDepth, pixelDepth\}}) \\
    \bottomrule
  \end{tabular}
  \caption{A complete list of events that are instrumented by PageGraph}.
  \label{table:instrumentation-points}
\end{table}
